# Supplementary material for: Asynchronous Federated Reinforcement Learning with Policy Gradient Updates: Algorithm Design and Convergence Analysis
Source: arXiv:2404.08003 source file (2025-01-23)
Supplement: Supplementary file 1 [file rebuttal.tex]

\section{Rebuttal}

\subsection{Summary}

Dear Chairs,

We greatly appreciate your time spent handling our paper. We have addressed all the reviewers' questions. We briefly summarize the discussion here, and hope this would help the evaluation.

--

1. Reviewer ``YjHR``

Mainly about theoretical settings and derivations.

- Algorithm Design and Derivation. We reformulated the algorithms with detailed explanations in Section 4, Page 7. We fixed the typos, and added explanations of derivations with details in Appendix B.

- Explanations of the Time Complexity. We added more explanations in Appendix A.1 and statements on Page 8, Line 392. It becomes more comprehensive and easier to understand.


%%%%%%%%%%%%%%%%%%%%%%%%%%%%%%%%%%%%%%%%%%%%%%%%%%%%%%%%%%%%%%
--

2. Reviewer ``T8LV``

Mainly about comparisons with previous works and the communication cost analysis.

- Contributions compared to the work of the Actor-Critic (not PG) method without General Policy Parameterization (not Deep RL) for the Global Convergence.

We added an extra discussion section in Appendix C.1 to address this concern. Beyond the general settings and differences above mentioned, we have a better convergence rate, and remove the impractical assumptions.

- Lack of Communication Complexity in FedRL. We added the analysis of communication cost in Appendix A.3 and highlighted our advantages.

- Questions about the agent index. We explained that the global convergence performance (boundary) on the server side has NO relationship with the agent index, and only depends on the average delay $\bar{\delta}$.

- Questions about the order of the theorems. We changed the orders as suggested.


%%%%%%%%%%%%%%%%%%%%%%%%%%%%%%%%%%%%%%%%%%%%%%%%%%%%%%%%%%%%%%
--

3. Reviewer ``KckT``

Mainly about comparisons with previous works.

- Novelty. 

    - We are the first work to analyze federated policy gradient methods with General Policy Parameterization, e.g., neural networks (Deep RL), for a Global Convergence, and achieve the SOTA results.

    - Even without the asynchronous setting, there is no previous FedPG work that achieves a global convergence with general policy parameterization with the SOTA rates.

    - Beyond that, we design the asynchronous method and further improve the performances, which is the main improvement and contribution in this paper.

- Comparison with a synchronous work without Global Convergence and General Function Parameterization. It only contains a momentum design without our delay-adaptive lookahead design.

    Except in the synchronous setting (previous works), there are several other main differences in terms of completeness and methodology:

    1. We achieve a **Global Convergence** with the SOTA rate, while that work (FedM for short) only focuses on stationary point convergence. It seems that FedM cannot go through the global convergence analysis without new techniques.

    2. We have **General Function Parameterization**, e.g., neural networks (Deep RL), results in both theory and experiments. That paper does not analyze the influence of general function parametrization, e.g., Deep RL, in theory. The general function approximation might bring higher sample complexity, especially for the global convergence.

    3. In their setting, the local policies will not be in different steps (Fixed to the hyperparameter $K$ in their paper). In our asynchronous setting, we do not require that each agent is in the same step, which brings the second-order error term in equation 31 and unbounded variance. Thus, we design the lookahead mechanism to cancel the second-order errors, normalized updates to bound the variance, and thus, secure the convergence. This technique is new and unique.

    4. Their momentum design is **NOT** the delay-adaptive lookahead method in our paper. 

        - The momentum method is used for gradient estimation (not sampling) at **Step 5** in Algorithm 1. We did not state this momentum part is a novelty in our method. Our delay-adaptive lookahead method is at **Step 8** in Algorithm 1 for trajectory ''sampling'' at Step 2 in Algorithm 2. This is new and has never been used before in any FedRL works. 

        - On the other hand, the orders are different. In momentum methods, the momented point is ''between'' the old ($k-1$)-th and the new $k$-th points. In our delay-adaptive lookahead method, the new point $k$-th is ''between'' the old ($k-1$)-th and the momented point. This is the reason that we call it ''lookahead''.

        - Roughly speaking, our method has two momentums. One (the gradient estimation one) is like the conventional momentum method. The other (the sampling one) is not and is technically new.


%%%%%%%%%%%%%%%%%%%%%%%%%%%%%%%%%%%%%%%%%%%%%%%%%%%%%%%%%%%%%%
--

4. Reviewer ``ui29``

Mainly about experiments.

- Communication Complexity Analysis. We added the analysis of communication cost and showed our advantages in Appendix A.3.

- Comparison when all algorithms converge. We added the experiments with long runs in Appendix A.3 to enhance our claims.


%%%%%%%%%%%%%%%%%%%%%%%%%%%%%%%%%%%%%%%%%%%%%%%%%%%%%%%%%%%%%%
--

5. Reviewer ``oswF``

Mainly about theoretical settings and derivations.

- Derivations Details, Clarifications, Explanations, and Typos in Section 4, Section 5, and Appendix B.

We fixed them accordingly, and explained each term in derivations in detail.



%%%%%%%%%%%%%%%%%%%%%%%%%%%%%%%%%%%%%%%%%%%%%%%%%%%%%%%%%%%%%%
% \subsection{Second Round}

% \textbf{Reviewer 3, KckT: 5}:

% We truly appreciate the responses.

% Here are the new results that we have added in the updated version as suggested:

% - Re-state the algorithms with clear explanations.

% - Time complexity analysis and explanations in Appendix A.1.

% - More explanations with details in the proof in Appendix B.

% - Reward performances with long runs in Appendix A.3.

% - Communication overhead analysis and comparisons between asynchronous and synchronous settings in Appendix A.3.

% We can further emphasize the key contribution points in the updated version. We briefly state here. We are the first work to analyze the policy gradient methods in FedRL with general function parameterization and achieve the SOTA global convergence rate. We improve the performances in communication cost and time consumption with an asynchronous setting, which is new.

% Do you have any specific aspects that we can clarify and further improve? Thank you so much for the suggestion!


% \textbf{Reviewer 4, ui29: 5}:

% We sincerely apologize for the confusion, and the claim before showing results. We did not include the partial results in the previous version. We have uploaded a new version, which includes the complete results in Appendix A.3. 

% In Appendix A.3, it contains descriptions with details. We briefly state here. For Swimmer-v4, Hopper-v4, and Walker2D-v4 tasks, PG achieves similar rewards with AFedPG in Figure 9. For Humanoid-v4, in some runs, PG achieves the reward, while in some runs, PG does not achieve the reward compared to our AFedPG, because of the hyperparameter tuning of PG, e.g., learning rates. 

% The hyperparameter tuning of PG has no contribution to our main claim. Recall that we aim to use these experiments to verify the speedup effect in AFedPG in Table 1. The suboptimal hyperparameters
% of PG in the Humanoid-v4 task do not influence the conclusion: The more agents in AFedPG, the faster the optimal reward will be achieved.

% Compared to the original version, we have added (1) Communication overhead analysis in Appendix A.3. (2) Reward performances with long runs. (3) More details in the proof, e.g., the derivation of equation 34 with details, and the explanation of equation 36. (4) Time complexity analysis in Appendix A.1. 

% We hope this would help to address the main concerns. Thank you for the re-evaluation based on the improvement under your suggestions.


% \subsection{First Round}

% \textbf{Reviewer 1, YjHR: 5}:

% Thank you for reading the paper carefully! If there are any other concerns, we would be happy to answer them.

% \textbf{W1.} 
% We are sorry about the confusion. In the original algorithms, the $k$ on the server and agent sides are not the same one. To avoid confusion, we have reconstructed the algorithm description (Algorithm 1 and 2), while keeping all notations unchanged in the theoretical analysis. In the new description, a simple plugin between the equations will lead to the theoretical results. We hope this could help.


% \textbf{W2.} Thank you so much for bringing this! It is indeed a typo. It should be $d_{k-1-\delta_{k-1}}$ instead of $d_{\delta_{k-1}}$. We have fixed the typo, and it should now be consistent.

% We have $e_{k} = d_{k - \delta_{k}} - \nabla J(\theta_{k})$ and $d_{k - \delta_{k}} = (1 - \alpha_{k - \delta_{k}}) d_{k-1 - \delta_{k-1}} + \alpha_{k - \delta_{k}} g(\widetilde{\tau}_{k - \delta_{k}}, \widetilde{\theta}_{k - \delta_{k}})$. Combining them, we have 
% $e_{k} = (1 - \alpha_{k - \delta_{k}}) d_{k-1 - \delta_{k-1}} - \nabla J(\theta_{k}) + \alpha_{k - \delta_{k}} g(\widetilde{\tau}_{k - \delta_{k}}, \widetilde{\theta}_{k - \delta_{k}})$. Then, we can have the result in \eqref{eq:e_k}, and construct the recursive form.



% \textbf{W3.} 
% In the worst case, the largest delay could be infinite (not communicate at all), while the average delay is upper bounded by $N$. 

% We have a very interesting result in AFedPG. We do not make any assumptions about the delay, and the largest delay is allowed to be infinite. If some agents do not communicate at all, we simply lose their computation resources. The convergence rate is upper bounded by the average delay $\bar{\delta}$, and the average delay is bounded by $N$ in Lemma B.10. In equation 37, the term with the average delay is much smaller than the dominated term $\mathcal{O}(K^{-2.5})$ ($K$ could reach an order of magnitude of six or even larger.), and thus, does not hurt the convergence rate.

% \textbf{W4.} Thank you for the suggestion! We have added the explanation with detailed derivation in Appendix A.1. It should be very easy to understand.

% \textbf{W5.} As the agent has the same computation requirement in each iteration (The number of collected samples is the same.), we assume that the time complexity in each iteration is the same. Sorry about the confusion. We have added this statement in line 388.

% %%%%%%%%%%%%%%%%%%%%%%%%%%%%%%%%%%%%%%%%%%%%%%%%%%%%%%%%%%%%%%
% \textbf{Reviewer 2, T8LV: 3}:

% \textbf{W1.} 
% The local update is a terminology in the conventional synchronous setting. In the asynchronous setting, the agent sends the update to the server as soon as it finishes the computation. In most conventional federated learning works, only the synchronous setting is considered. We aim to extend it to the asynchronous setting.


% \textbf{W2.} 
% Thanks for the suggestion! First, we admit that [3] contains novel contributions in theoretical analysis. 
% % However, their result is not ''accurate'' (See W3). 
% However, it only includes linear parametrization, which is a very weak and unpractical result (See W3). With a general function parametrization, e.g., neural networks (Deep RL), the SOTA result of the AC method is $\mathcal{O}({\epsilon}^{-3})$ [4]. It is worse than the SOTA result in policy gradient, which is $\mathcal{O}({\epsilon}^{-2.5})$. We aim to compare with the best results, and thus, choose to analyze policy gradient methods.

% [4] Closing the Gap: Achieving Global Convergence (Last Iterate) of Actor-Critic under Markovian Sampling with Neural Network Parametrization. ICML 2024.


% \textbf{W3.} 

% % First, though [3] claims to have global convergence results, the theoretical results in [3] are not ``accurate''. Theorem 2 and 4 in [3] are NOT global convergences. They are FOSP. The correct criterion of the global convergence is shown in Theorem 1 in [4], and Equation 2.3 and Theorem 4.6 in [5].

% First, [3] only has Linear parametrization, which is a very weak result with limited meaning. With a General Function Parametrization, e.g., neural networks (Deep RL), there is no such a result. We consider a general and practical setting with a general function parametrization. Even in the single-agent setting (without federated agents), the SOTA result of the AC method is $\mathcal{O}({\epsilon}^{-3})$ [4], which is still worse than our $\mathcal{O}({\epsilon}^{-2.5})$. In the federated setting, there is no result that achieves $\mathcal{O}({\epsilon}^{-3})$ for AC methods. With a general function parameterization, we compare the performances in Figure 4 with this method.

% Second, [3] relies on a strong and unpractical assumption, Assumption 2. It assumes that the largest delay is bounded by a constant $K_{0}$. However, in practice, the slowest agent may not communicate with the server, and thus, has an infinite delay. In our analysis, we do not require any boundary for the largest delay, because we only contain the average delay in the convergence rate, and the average delay is naturally bounded by the number of agents $N$ in Lemma B.10 (our corollary).

% Third, [3] is an AC method with extra value networks, which requires much more computation and memory cost compared to the pure policy gradient method. Thus, the fine-tuning of Gemini and GPT4 uses policy gradient methods instead of AC methods.

% % [5] An Improved Analysis of (Variance-Reduced) Policy Gradient and Natural Policy Gradient Methods. NeurIPS 2020.

% \textbf{Q4.} 

% We aim to train a global policy in FedRL. The theorems give the convergence rates for the policy model w.r.t. the number of global updates on the server. It has no relationship with the index of agents. We achieve a result that the global convergence rate is upper bounded by the average delay, and the average delay is bounded by the number of agents $N$. This is new in FedRL. If there are any other questions, we would be happy to answer them.

% \textbf{Q5.}

% We are the first work to analyze federated policy gradient methods with General Policy Parameterization, e.g., neural networks (Deep RL), for a Global Convergence, and achieve the SOTA results. 

% Even without the asynchronous setting, there is NO previous FedPG work that achieves a Global convergence with general policy parameterization (Deep RL) with the SOTA rates.

% Beyond that, we design the asynchronous method and further improve the performances, which is the main improvement in this paper.


% \textbf{Q6.} 
% Thank you for the suggestion. We have changed the order in the main paper.



% %%%%%%%%%%%%%%%%%%%%%%%%%%%%%%%%%%%%%%%%%%%%%%%%%%%%%%%%%%%%%%
% \textbf{Reviewer 3, KckT: 5}:

% \textbf{W1.} 
% We are the first work to analyze federated policy gradient methods with general policy parameterization, e.g., neural networks (Deep RL), for a Global convergence, and achieve the SOTA results. 

% Even without the asynchronous setting, there is no previous FedPG work that achieves a global convergence with general policy parameterization with the SOTA rates.

% Beyond that, we design the asynchronous method and further improve the performances, which is the main improvement in this paper.

% We also list 4 points in W2, which makes the novelty more clear and easy to understand. If there are any other concerns, we would be happy to answer them.


% \textbf{W2.} 
% Thank you for bringing this work! We have cited it in the updated version as it has valuable analysis and improves the results in FedRL. However, there are several main differences in terms of completeness and methodology:

% 1. We achieve a Global Convergence with the SOTA rate, while that work (FedM for short) only focuses on stationary point convergence. It seems that FedM cannot go through the global convergence analysis without further techniques.

% 2. We have general function parameterization, e.g., neural networks (Deep RL), results in both theory and experiments. That paper does not analyze the influence of general function parametrization, e.g., deep RL, in theory. The general function approximation might bring higher sample complexity, especially for the global convergence.

% 3. In their setting, the local policies are not in different steps (Fixed to the hyperparameter $K$ in their paper). In our asynchronous setting, we do not require that each agent is in the same step, which brings the second-order error term. Thus, we design the lookahead mechanism to cancel the errors, and secure the convergence. This technique is new and unique.

% 4. Their momentum design is NOT the delay-adaptive lookahead method. The momentum is used for gradient estimation (not sampling) at Step 3 in Algorithm 2. We did not state this momentum part is a novelty in our method. Our delay-adaptive lookahead method is at Step 7 in Algorithm 1 for trajectory ``sampling'' at Step 2 in Algorithm 2. This is new and has never been used before in any FedRL works. 

% On the other hand, the orders are different. In momentum methods, the momentumed point is ``between'' the old ($k-1$)-th and the new $k$-th points. In our delay-adaptive lookahead method, the new point $k$-th is ``between'' the old ($k-1$)-th and the momentumed point. It is the reason that we call it ``lookahead''.
% Roughly speaking, we have two momentums, but unlike the definition of the momentum gradient descent, the sampling one is not a conventional momentum.



% %%%%%%%%%%%%%%%%%%%%%%%%%%%%%%%%%%%%%%%%%%%%%%%%%%%%%%%%%%%%%%
% \textbf{Reviewer 4, ui29: 5}:

% \textbf{W1.} 
% Thank you so much for this suggestion! The communication overhead was not the target of this paper. However, after we accepted your valuable advice and dived deep into the analysis, we find that AFedPG actually has advantages compared to FedPG. We added communication overhead results in Appendix A.3, and answered Q3. We hope this could address your concerns.

% \textbf{W2.} 
% Thank you! We have fixed the typos with another round of proofreading.


% \textbf{Q1.}
% In the asynchronous setting, concurrency roughly means the number of machines that are computing. In the synchronous setting, the server waits until it receives policy gradients from all $N$ agents, while in the asynchronous setting, the server runs as soon as one policy gradient is received. In a continuous space (time), it has measure zero that two discrete time spots are the same. Thus, only one agent applies.


% \textbf{Q2.} 
% It takes a very long time to wait for them to converge to the optimal point, especially when the state and action spaces are large. We only use these experiments to show the benefit of more agents. To answer the question and verify this hypothesis, we test the result on the Swimmer-v4 task. They can converge to a similar reward, while the variance (shadow area) is larger. We assume the federated setting has the potential ability to reduce the variance when more agents engage, which could be an interesting direction for future study.


% \textbf{Q3.} 
% Thank you for the suggestion! We have added the analysis of experiments in Appendix A.3 to further enhance it. We briefly state the key points here.

% In theory, the synchronous setting and asynchronous settings have the same cumulative communication cost as the sample complexities are the same, and each agent collects the same amount of samples in each update. Our analysis shows that the AFedPG could keep the SOTA sample complexity in policy gradient methods in RL in Table 1. Moreover, when we analyze the training process through the lens of fine-grained time, AFedPG shows several advantages.

% On the server side, in FedPG, it is noticeable that the communication mainly happens in a short time window in the downlink process, which brings a heavy burden with a peak, especially in the resource constraint scenario. In AFedPG, the communication is more evenly distributed, which does not have a peak burden and has less requirement for communication resources.

% On the agent side, in FedPG, all agents have the same communication burden. In AFedPG, the leader agent (fast) has more communication burden $\mathcal{O}(t_{\max})$, while the straggler agent (slow) has less communication burden $\mathcal{O}(t_{\min})$. This is a more rational allocation compared to the equality setting regardless of the heterogeneous computing resources. In practice, agents have heterogeneous resources, while FedPG does not consider this and evenly distributes the burden. The equal allocation could bring too much burden for the slow ones. In AFedPG, it shifts the burden to the fast ones naturally.


% %%%%%%%%%%%%%%%%%%%%%%%%%%%%%%%%%%%%%%%%%%%%%%%%%%%%%%%%%%%%%%
% \textbf{Reviewer 5, oswF: 6}:

% Thank you for reading the paper carefully! If there are any other concerns, we would be happy to answer them.

% \textbf{W1.} Section 4.

% We add more explanation in $d_{k-1}$ and $\theta_{k-1}$, and restate our algorithms to clearly show the process.

% We have added literature explanations.

% For trajectory sampling, it is indeed not practical to sample the whole trajectory. However, with the discount factor $\gamma$, the variance is exponentially small in the horizon [1,2]. The truncation does not influence the convergence results, and thus, the infinite horizon setting [3] is widely used in the recent analysis.


% \textbf{W2.} Section 5.

% Thank you for the remainder! Though the equations are correct in the theorems in the appendix, we had a typo in its simplified version in equation 10. We have fixed the typo in the main paper.

% We have added the derivation with details in Appendix A.1. The line 394 could be well explained.


% \textbf{W3.} Appendix B.

% Thanks for the suggestion! We have added the explanations of the conventional notations in Appendix B.1.

% We have added the exact positions of the cited lemmas.

% We have fixed all typos with more rounds of proofreading.


% [1] On the Theory of Policy Gradient Methods: Optimality, Approximation, and Distribution Shift. Journal of Machine Learning Research 2021.

% [2] An Improved Analysis of (Variance-Reduced) Policy
% Gradient and Natural Policy Gradient Methods. NeurIPS 2020.

% [3] Improved Sample Complexity Analysis of Natural Policy Gradient Algorithm with General Parameterization for Infinite Horizon Discounted Reward Markov Decision Processes. AISTATS 2024.
